# Supplementary material for: End-to-End Multimodal Fact-Checking and Explanation Generation: A Challenging Dataset and Models
Source: arXiv:2205.12487 source file (2023-07-06)
Supplement: Supplementary file 1 [file 8appendix.tex]

% \appendix
%  \newpage
% \section{Supplementary Material}

% \section{Appendix}
% \subsection{Comparison with Previous Datasets}

% Table~\ref{tab:compare} compares \dataset{} with other existing datasets for fack-checking and misinformation detection.
 
% \begin{table}[!htp]
 
% \small
% \renewcommand{\thetable}{5}
% \centering
% \resizebox{\columnwidth}{!}{%
% \begin{tabular}{p{3.9cm}|p{1.25cm}<{\centering}|p{1.4cm}<{\centering}|p{1.9cm}<{\centering}|p{1.2cm}<{\centering} |p{1.4cm}<{\centering}  }
% \toprule
% \diagbox{\textbf{Dataset}}{\textbf{Feature}}  &\textbf{Evidence Retrieval} & \textbf{Multimodal} & \textbf{Explainable Fact-checking} &  \textbf{Annotated Label} &\textbf{Annotated Evidence} \\
%  \midrule
% FEVER~\cite{Thorne}  &  \cmark & \xmark & \xmark&  \cmark&  \cmark
% \\
% Liar~\cite{Wang} & \xmark &\xmark& \xmark& \cmark & \cmark
% \\
% \cite{Hanselowski} & \cmark & \xmark & \xmark& \cmark & \cmark
% \\
% PUBHEALTH~\cite{Kotonya}  & \cmark & \xmark & \cmark& \cmark & \cmark
% \\
% FACTIFY~\cite{Mishra2021} & \xmark & \cmark & \xmark& \xmark & \xmark
% \\
% MuMiN ~\cite{Nielsen} & \xmark & \cmark   & \xmark &\cmark  & \xmark
% \\
% FakeNewsNet~\cite{Shu}& \cmark & \cmark & \xmark& \cmark & \xmark
% \\
% Fauxtography~\cite{Zlatkova} & \xmark & \cmark & \xmark&  \cmark & \xmark
% \\ 
% NewsBag~\cite{Jindal2020} & \xmark & \cmark & \xmark& \cmark & \xmark
% \\
% QProp~\cite{Barron-Cedeno2019} & \xmark & \cmark & \xmark& \cmark & \xmark
% \\
% TABFACT~\cite{Chen_TABFACT} & \xmark & \cmark & \xmark& \cmark & \cmark
% \\
% CLAIMDECOMP~\cite{Chen} & \cmark & \xmark &  \cmark& \cmark  & \cmark 
% \\
% MultiFC~\cite{Augenstein} & \cmark&\xmark   & \xmark& \cmark & \xmark
% \\
% FEVEROUS~\cite{Aly} & \cmark&  \xmark  & \xmark&  \cmark & \cmark 
% \\


% \midrule
% \textbf{\dataset{} (Ours)} & \cmark & \cmark & \cmark&  \cmark  &  \cmark 
% \\ 

% \bottomrule
% \end{tabular}%
% }
 
% \caption{Comparison between \dataset{} and other related datasets. The columns indicate whether the dataset requires automatic evidence retrieval, multimodal reasoning or explanation generation, whether its label and evidence are annotated by human.
% %\lifu{can we add more columns for comparison?}\menglong{I will add them this morning}\lifu{make it clearer the meaning of each column. e.g., what does the Evidence column mean?}\menglong{Done. Do their works contains evidence retrieval phase? Are their fact-checking in a explanable manner, like providing some hints or explanations about their judgements? Is it multimodal?   }  
% }
% \label{tab:compare}
 
% \end{table}
 

% \menglong{We can add the following information in the supplementary material. }

% \subsection{Experiment Analysis} 
% \label{appe:experiment analysis}

% Figure~\ref{fig:discussion example} shows several examples to illustrate the challenges for multimodal claim verification.

%  \begin{figure*}[!htp]
%     \renewcommand{\thefigure}{4}
%     \centering
%     \includegraphics[width=1\linewidth]{figures/Mocheg_discussion_examples.pdf}%0.9
%     \caption{Examples of Multimodal Fact Checking. The \textit{Truthfulness} column shows gold labels. %\lifu{The evidence text in \#5 seems unrelated.}\menglong{Done}  \lifu{Also, claim \#7 reaffirms one of my concerns about this dataset, that the claims/ evidence might be missing context. The claim says "No One Realizes How Dangerous This Popular Vacation Spot in California Actually Is". It's unclear what is this spot and therefore how to fact check this claim. Human performance or quality analysis on the proposed dataset might shed some light here.}\menglong{Done. Replaced \#7. }
%     }
%     \label{fig:discussion example}
% \end{figure*}



% \subsection{Access to the dataset} 
%\lifu{Are these required by AAAI? if not, we need to remove all these statements. Also, the url definitely violates the double-blind policy.}\menglong{Have removed our links. I am adding documents for AAAI}
% The \dataset{} dataset can be accessed from \url{http://nlplab1.cs.vt.edu/~menglong/project/multimodal/fact_checking/MOCHEG/dataset/}. Elementary code to process the data and run baseline experiments will be publicly available on the Github repository \url{https://github.com/VT-NLP/Mocheg}. The new version of our dataset will also be notified in this Github repository. The authors of this paper will ensure proper long-term maintenance and access to the dataset. The DOI is 10.5281/zenodo.6653771\footnote{\url{https://doi.org/10.5281/zenodo.6653771}}. Structured metadata in the \textit{schema.org}\footnote{\url{http://schema.org/}} format is accessed from our server \footnote{\url{http://nlplab1.cs.vt.edu/~menglong/project/multimodal/fact_checking/MOCHEG/homepage.html}}


% \subsection{Dataset Format}
% Our dataset is split into training, development, test subsets, and a collection of documents and images as the source of evidence:
% \begin{enumerate}
% \item Text collection named ``Corpus3.csv'', which contains the articles as the sources for the text evidence retrieval task; Each entry stands for one document and consists of three key fields:
%     \begin{enumerate}
%             \item  relevant\_document\_id: The ID of the document in the text collection
%             \item  claim\_id: The ID of the claim which is relevant to this document
%             \item  Origin Document: The document content.  Its usage is as follows:                     \begin{enumerate}  
%                                 \item Input (collection) for the text evidence retrieval task
%                             \end{enumerate}
            
%     \end{enumerate}

% \item The image collection is saved in the ``images'' folder, which contains all images as the sources for the image evidence retrieval task. Each image is named in the format ``@claim\_id-@relevant\_document\_id-@img\_id-@description''.  Its usage is as follows:                     
%     \begin{enumerate}  
%                     \item Input (collection) for the image evidence retrieval task
%     \end{enumerate}
% \item Training subset, saved in the  ``train'' folder, which contains the following items:
%     \begin{enumerate}
%         \item  ``Corpus2.csv'', which contains the claim, text evidence, truthfulness label for the claim verification task, and ruling outline, which explains the reasoning and ruling process and is used for the explanation generation task. Each entry stands for one piece of evidence. If there are multiple pieces of evidence for one claim, there will be multiple rows for this claim. In detail, it contains the following key fields:
%         \begin{enumerate}     
%                     \item  Claim: The claim content we need to check the truthfulness. Its usage is as follows: 
%                         \begin{enumerate}  
%                             \item Input (query) for the evidence retrieval task
%                             \item Input for the claim verification task
%                             \item Input for the explanation generation task
%                         \end{enumerate}
%                     \item  claim\_id
%                     \item Evidence: One piece of text evidence that is relevant to this claim. It records the ground truth text evidence in the text evidence retrieval task. It can be retrieved from the text collection. Its usage is as follows: 
%                         \begin{enumerate}  
%                             \item Ground truth text for the text evidence retrieval task
%                             \item Input for the claim verification task
%                             \item Input for the explanation generation task
%                         \end{enumerate}
%                     \item evidence\_id: The ID of the evidence
%                     \item cleaned\_truthfulness: The truthfulness label (i.e., \textit{support}, \textit{refute} and \textit{not enough information}). Its usage is as follows: 
%                         \begin{enumerate}  
%                             \item Ground truth for the claim verification task
%                             \item Input for the explanation generation task
%                         \end{enumerate}
%                     \item ruling\_outline: It is a short paragraph to explain the reasoning and ruling process. Its usage is as follows: 
%                         \begin{enumerate}  
%                             \item Ground truth for the explanation generation task
%                         \end{enumerate}
%                     \item Origin: It is the ruling article on the fact-checking websites. The ruling\_outline can be seen as the summarization of the Origin.
%                     \item Snopes URL: The url for the corresponding fact-checking article
%         \end{enumerate}
%         \item  ``images'' folder, which contains the image evidence that is relevant to the claims in the training subset. It records the ground truth image evidence in the image evidence retrieval task. They can be retrieved from the image collection. Each image is named in the format ``@claim\_id-proof-@img\_id-@description''.   Its usage is as follows: 
%                         \begin{enumerate}  
%                             \item Ground truth images for the image evidence retrieval task
%                             \item Input for the claim verification task
%                             \item Input for the explanation generation task
%                         \end{enumerate}
       
%         \item ``text\_evidence\_qrels\_sentence\_level.csv''. It records the ID of the ground truth sentence in the text evidence retrieval task. It is in the trec qrel\footnote{\url{https://trec.nist.gov/data/qrels_eng/}} format with four fields:
%             \begin{enumerate}     
%                 \item TOPIC: In our case, it is the claim id
%                 \item ITERATION: Constant 0, no special meaning
%                 \item DOCUMENT\#: In our case, it is the corpus id which is in the format ``@claim\_id-@relevant\_document\_id-@sentence\_id''
%                 \item RELEVANCY: 1 for relevant and 0 for irrelevant
%             \end{enumerate}
%         \item ``text\_evidence\_qrels\_article\_level.csv''. It records the ID of the ground truth article in the text evidence retrieval task. Its format is similar to the trec qrel format, and it has five fields:
%             \begin{enumerate}     
%                 \item TOPIC: In our case, it is the claim id
%                 \item ITERATION  
%                 \item DOCUMENT\#: In our case, it is the relevant\_document\_id  
%                 \item RELEVANCY: 1 for relevant and 0 for irrelevant
%                 \item evidence\_id: Since we have saved the ground truth text evidence in the ``Corpus2.csv'' in the training, development, and test datasets, we add the corresponding evidence\_id here.
%             \end{enumerate}
%         \item ``img\_evidence\_qrels.csv''. It records the ID of the ground truth image in the image evidence retrieval task. Its format is similar to the trec qrel format, and it has five fields:
%             \begin{enumerate}     
%                 \item TOPIC: In our case, it is the claim id
%                 \item ITERATION  
%                 \item DOCUMENT\#: In our case, it is the image name in the image collection 
%                 \item RELEVANCY: 1 for relevant and 0 for irrelevant
%                 \item evidence\_id: Since we have saved the ground truth image evidence in the ``images'' folder in the training, development, and test datasets, we add the corresponding image name here.
%             \end{enumerate}
%     \end{enumerate}

% \item Development subset, saved in the  ``val'' folder. The format is same with Training subset
% \item Test subset, saved in the  ``test'' folder. The format is same with Training subset
% \item supplementary folder. This folder contains some objects which are optional for the dataset. All supplementary objects can be generated by the scripts in our Github repository, but the generation may take several hours. To make the process smooth, we include these side products in the dataset.
%     \begin{enumerate}  
%         \item Corpus3\_sentence\_level.csv: We split the documents in the ``Corpus3.csv'' into sentence level and store them in this file. It has five fields: 
%             \begin{enumerate}  
%             \item claim\_id
%             \item relevant\_document\_id
%             \item paragraph\_id: The ID for this sentence. Although this field is for just one sentence currently, it is called ``paragraph\_id'' to support the future work where we can merge several sentences into one paragraph for our experiments.
%             \item corpus\_id: It is in the format ``@claim\_id-relevant\_document\_id-@paragraph\_id''
%             \item paragraph: The sentence content.
%             \end{enumerate}
%         \item img\_corpus\_emb.pkl: The embedding for the image collection, encoded by ``clip-ViT-B-32'' checkpoint \footnote{\url{https://www.sbert.net/docs/pretrained_models.html}}.
%     \end{enumerate}
    
% \end{enumerate}    


% \subsection{Intended use}
% The dataset can be used for end-to-end multimodal fact-checking and explanation generation task, where the system needs to sequentially or jointly perform all three sub-tasks, including {\em multimodal evidence retrieval}, {\em multimodal claim verification}, and {\em multimodal explanation generation}.

% The dataset can also be used directly for these three sub-tasks separately.

% The dataset can also be used in the unimodal setting, like text-only explanation generation.


% \subsection{Data Statement}
% We follow the data statement structure of \cite{bender2018data} to give additional insights into the dataset. The \dataset{} consists of 21,184 claims where each claim is annotated with a truthfulness label and ruling statement, with 43,148 text evidence and 15,373 image evidence. We describe the dataset construction process in Section 3 in our paper. 
% \subsubsection{Curation Rationale}
% PolitiFact and Snopes are two widely used websites to fight against the spreading of misinformation, where journalists are asked to manually check and verify each claim and write a ruling article to share their judgment. Considering this, we use these two websites as the data sources and crawl all claims from these websites. We then remove some claims which do not contain evidence.
% \subsubsection{Language Variety} The content in our dataset is in US (en-US) mainstream Englishes.
% \subsubsection{Speaker Demographic}  It is expected that most of the speakers speak English as a native language. Our data source focuses on political topics.
% \subsubsection{Annotator Demographic} The journalists in Politifact and Snopes provide the annotations. However, their personal information, like gender, and age, is not directly available on the websites.
% \subsubsection{Speech Situation} Generally, the claims are from online speeches, public statements, news articles, and social media platforms, such as Facebook, Twitter, Instagram, TikTok, and so on. 
% \subsubsection{Content Characteristics} Our dataset is a multi-modal dataset with text and images.





% \subsection{Author Statement and Licensing}
% We bear all responsibility in case of violation of rights. Our dataset is licensed under the CC BY 4.0\footnote{\url{https://creativecommons.org/licenses/by/4.0/}}. The associated codes to \dataset{} for data crawler and baseline are licensed under Apache License 2.0\footnote{\url{https://www.apache.org/licenses/LICENSE-2.0}}. 

% These data annotations incorporate material from Politifact and Snopes, which is licensed pursuant to the Politifact Copyright Policy\footnote{https://www.politifact.com/copyright/} and Snopes Copyright Policy \footnote{https://www.snopes.com/terms-and-conditions/}. Our data crawler scripts are based on the conll2019-snopes-crawling repository \footnote{\url{https://github.com/UKPLab/conll2019-snopes-crawling}}, which is under Apache License 2.0. In our experiments, we applied information retrieval models\footnote{\url{https://github.com/UKPLab/sentence-transformers}} and text generation model\footnote{\url{https://github.com/huggingface/transformers}}, which are under Apache License 2.0. We referred to the controllable generation model\footnote{\url{https://github.com/laihuiyuan/pre-trained-formality-transfer}}~\cite{Lai2021}, which is under MIT License\footnote{\url{https://github.com/laihuiyuan/pre-trained-formality-transfer/blob/main/LICENSE}}.


% \subsection{Ethics Statement}
% We carefully follow the ethics guidelines \footnote{\url{https://neurips.cc/public/EthicsGuidelines}} and have not found potential societal impacts so far. Our work can be used to fact-check and stop the spread of misinformation. Our dataset does not use features or label information about sensitive personally identifiable information, like individual names.

% Since our dataset contains internet claims, some claims may be offensive. However, we crawl the articles from some reputational fact-checking websites, like Politifact and Snopes, to decrease the possibilities for offensive content.

% \subsection{Reproducible Result}
% All checkpoints will be made publicly available in our website. The results in the paper can be reproduced with these checkpoints.
% in the checkpoint folder \footnote{\url{http://nlplab1.cs.vt.edu/~menglong/project/multimodal/fact_checking/MOCHEG/checkpoint}}. 


% \barry{Desk Rejection Policy: Figures, tables, proofs, appendixes, acknowledgements, or any other content after page 9 of the submission.}
% \barry{Appendix section should be at the end of our paper after the References page. However, in that case, the appendix will appear after page 9, which may trigger the desk rejection. Should we just move A.2 Fact-checking Process section into the main paper following the ETHICAL STATEMENT section and remove A.1 Experiment Setting section? }
% \barry{I have merged A.2 Fact-checking Process section into Ethical Statement and A.1 Experiment Setting section into the Experiment section}
% \subsection{Experiment Setting}
% We use 2 Quadro RTX 8000 to run our experiments. The retrieval models cost 15 GB and are trained for about 20 runs with a batch size of 256. The claim verification models cost 3 GB and are trained for about 50 runs with a batch size of 128. The explanation generation model costs 45 GB and is trained for about 30 runs with a batch size of 10. We use grid search to tune the hyperparameters which are shown in Table~\ref{tab:hyperparameter}.
% %The values tried for key hyperparameters are shown in Table~\ref{tab:hyperparameter}.



% % %current table for retrieval
% \begin{table}[!htp]%{r}{0.7\textwidth}
% % \vspace{-7mm}
% \renewcommand{\thetable}{6}
% \centering
% %\lifu{what does cosine mean? what does rerank mean??}\menglong{Done. Has edited to ``w/ re-ranking module setting'' and ``w/o re-ranking module setting''}
% \footnotesize
% %\resizebox{0.9\columnwidth}{!}{%
% \resizebox{ \columnwidth}{!}{
% \begin{tabular}{l|c|c }
% \toprule
%   \textbf{Model}  & \textbf{Learning Rate}&\textbf{Batch Size}  \\
% \midrule
%  Claim Verification &0.1, 0.01, 0.001, 0.0001 & 64, 128, 256, 512, 1024, 2048\\
%  Evidence Retrieval & 0.00001, 0.000001, 0.0000001& 256, 480, 512 \\
%  Explanation Generation & 0.05, 0.0005, 0.00005&10, 12, 48, 192 \\
% \bottomrule
% \end{tabular}%
% }
% \caption{Search space of hyperparameters for the models of three subtasks.}
%  \label{tab:hyperparameter}
% \end{table}


 

% \subsection{Fact-checking Process in Snopes and Politifact}
% \label{appendix_fact_checking}
% We introduce the fact-checking process of Snopes and Politifact to show why our data sources are reliable and unbiased.
% According to Politifact\footnote{ \url{https://www.politifact.com/article/2018/feb/12/principles-truth-o-meter-politifacts-methodology-i/}} and Snopes\footnote{\url{https://www.snopes.com/transparency/}}, they always attempt to contact the person, website, or organization that made the statement they are fact-checking. They will have consultations with a variety of expertise. They seek direct access to government reports, academic studies, and other data. They also have one to two rounds of reviews. Finally, they will accept the error correction from the public and mark the corrected articles. 

% According to Politifact, PolitiFact journalists avoid the public expression of political opinion and public involvement in the political process to set their own opinions aside as they work to uphold principles of independence and fairness. 23 of 36 journalists are women. According to Snopes, members of their editorial staff are precluded from donating to or participating in, political campaigns, political party activities, or political advocacy organizations. 6 of 10 journalists are women.

% \subsection{Copyright and Dataset Sharing Plan}
